# Supplementary material for: DES-LOC: Desynced Low Communication Adaptive Optimizers for Training Foundation Models
Source: arXiv:2505.22549 source file (2025-05-28)
Supplement: Supplementary file 1 [file notation-table.tex]

\clearpage
% -------------------- % 
\section{Notation Table}
% -------------------- %

\begin{table}[!h]
\caption{Notation we use throughout the paper.}
\label{tbl:notation}
\begin{center}
\begin{tabular}{|c|l|}
\hline % ------------------------------------------------ %
\multicolumn{2}{|c|}{{\bf Basic} }\\
\hline % ------------------------------------------------ %
$d$ & number of the model parameters to be trained \\
\hline
$M$ & number of the machines/workers in distributed system \\
\hline
$N$ & number of optimizer states, e.g., SGD ($N=0$), SGDM ($N=1$), Adam/ADOPT ($N=2$) \\
\hline
$t$ & time step or iteration counter \\
\hline
$m$ & machine index, $m\in\{0,1,\dots,M-1\}$ \\
\hline
$\eta_t$ & learning rate or step size \\
\hline
$x_t$ & parameters/weights of the model, optimization variable \\
\hline
$\xi_t$ & stochastic mini-batch sample of data \\
\hline
$u_t,\; v_t$ & first and second order momentum variables of Adam \\
\hline
$\beta_1,\; \beta_2$ & first and second order momentum parameters of Adam \\
\hline
$\rho$ & clipping threshold \\
\hline
$K_x,\;K_u,\;K_v$ & number of local steps per communication round for each variable \\
\hline
$R$ & total communication rounds \\
\hline
$T$ & total number of optimization steps \\
\hline
$-$ & - \\
\hline
$-$ & - \\
\hline
$-$ & - \\
\hline
$-$ & - \\
\hline
$-$ & - \\
\hline
$-$ & - \\
\hline
\hline % ------------------------------------------------ %
\multicolumn{2}{|c|}{{\bf Standard} }\\
\hline % ------------------------------------------------ %
$-$ & - \\
\hline
\hline % ------------------------------------------------ %
\multicolumn{2}{|c|}{{\bf More} }\\
\hline % ------------------------------------------------ %
$-$ & - \\
\hline
$-$ & - \\
\hline
$-$ & - \\
\hline
\end{tabular}
\end{center}
\end{table}
