# Supplementary material for: DES-LOC: Desynced Low Communication Adaptive Optimizers for Training Foundation Models
Source: arXiv:2505.22549 source file (2025-05-28)
Supplement: Supplementary file 2 [file other_related_work.tex]

\section{Other Related Work}
\paragraph{Federated Adaptive Optimizers.} Early attempts at bringing adaptivity to federated approaches, such as FedOPT\~\citep{FedOPT}, attempted to get around this limitation by using SGD at each worker and operating on pseudo-gradients calculated at round boundaries, the difference between model parameters at the start and end of a round, rather than gradients. However, this does not help stabilize worker training locally and has not been successfully applied for large-scale pre-training of foundation models.
