# Supplementary material for: DES-LOC: Desynced Low Communication Adaptive Optimizers for Training Foundation Models
Source: arXiv:2505.22549 source file (2025-05-28)
Supplement: Supplementary file 3 [file wall_time_modeling_revised.tex]

* 
            *
